# Supplementary material for: The Order of Things: Position-Aware Network-friendly Recommendations in Long Viewing Sessions
Source: arXiv:1905.04947 source file (2019-05-13)
Supplement: Supplementary file 1 [file appendixA.tex]

\myitem{Proof for inequality (\textit{c})}.
The optimal vectors of the Lagrangian $(\mathbf{z}^{\ast},\mathbf{w}^{\ast},\mathbf{F}^{\ast},\boldsymbol{\lambda}_1^{\ast},\boldsymbol{\lambda}_2^{\ast})$ define a saddle point for $\mathcal{L}_{0,0}$ for which we have 
\begin{align}
\mathcal{L}_{0,0}(\mathbf{z}^{\ast},\mathbf{w}^{\ast},\mathbf{F}^{\ast},\boldsymbol{\lambda}_1^{\ast},\boldsymbol{\lambda}_2^{\ast}) \le \mathcal{L}_{0,0}(\mathbf{z}^{k+1},\mathbf{w}^{k+1},\mathbf{F}^{k+1},\boldsymbol{\lambda}_1^{\ast},\boldsymbol{\lambda}_2^{\ast}). 
\end{align}

Taking also into account that at the optimal point it holds (a) $\mathbf{z}^{\ast} - \mathbf{F}^{T(\ast)} \cdot \mathbf{1} = \mathbf{p}_0$ and (b) $\mathbf{z}^{\ast} = \mathbf{w}^{\ast}$, the primal residuals at the left handside (LHS) of the inequality are driven to zero. Having also defined $p^{\ast} = \mathbf{z}^{T(\ast)}\cdot \mathbf{c}$ returns the claimed inequality.

% \theo{I will denote the $z^{\prime}$ as $w$, since this is how I had it in my notes during summer and further having the prime z, may lead to having three superscripts which looks seriously ugly/confusing.}

\myitem{Proof for inequality (\textit{b})}.
According to the definition, the vector $\mathbf{z}^{k+1}$ minimizes $\mathcal{L}_{\rho_1,\rho_2}(\mathbf{z},\mathbf{w}^{k},\mathbf{F}^{k})$. The function $f(\mathbf{z}) = \mathbf{z}^{T}\cdot \mathbf{c} + \mathbf{I}_{\mathcal{S}}(\mathbf{z})$ is closed proper and convex, so is $\mathcal{L}_{\rho_1,\rho_2}$ and its subgradient is $\partial f (\mathbf{z}) = \mathbf{c} + \partial \mathbf{I}_{\mathcal{S}} (\mathbf{z})$. The optimality condition is 
\begin{align} \label{optimalityCon11}
0 \in \partial \mathcal{L}_{\rho_1,\rho_2}(\mathbf{z}^{k+1},\mathbf{w}^{k},\mathbf{F}^{k},\boldsymbol{\lambda}_{1}^{k},\boldsymbol{\lambda}_{2}^{k}) = \partial f (\mathbf{z}^{k+1})  
+ \boldsymbol{\lambda}_{1}^{k}+ \\ \nonumber + \boldsymbol{\lambda}_{2}^{k}  + \rho_1(\mathbf{z}^{k+1} - \mathbf{F}^{T(k)} \cdot \mathbf{1} - \mathbf{p}_0) + \rho_2 (\mathbf{z}^{k+1} - \mathbf{w}^{k})
\end{align}

Our multipliers' updates give the following useful respective expressions $\boldsymbol{\lambda}_{1}^{k} = \boldsymbol{\lambda}_{1}^{k+1} - \rho_1 \mathbf{r}_{1}^{k+1}$, $\boldsymbol{\lambda}_{2}^{k} = \boldsymbol{\lambda}_{2}^{k+1} - \rho_2 \mathbf{r}_{2}^{k+1}$. If we also plug at the respective $\mathbf{r}_i^{k+1}$ the appropriate expression at the $(k+1)$-th time instant and combine with Eq.(\ref{optimalityCon11}), we end up with the following 

\begin{align} \label{optimalityCon12}
0 \in \partial f (\mathbf{z}^{k+1}) +  \boldsymbol{\lambda}_{1}^{k+1} + \rho_1(\mathbf{F}_{k+1}^{T} - \mathbf{F}_{k}^{T})\cdot \mathbf{1} \\ \nonumber
\boldsymbol{\lambda}_{2}^{k+1} +  \rho_2(\mathbf{w}^{k+1} - \mathbf{w}^{k})
\end{align}

The expression of Eq.(\ref{optimalityCon12}) suggests that 

\begin{align} \label{z_alsoMinimizes}
\mathbf{z}^{k+1} = \underset{\mathbf{z}}{\operatorname{argmin}}\{f(\mathbf{z})+\boldsymbol{\lambda}_{1}^{k+1}+\boldsymbol{\lambda}_{2}^{k+1}+ \\ \nonumber
\rho_1(\mathbf{F}_{k+1}^{T} - \mathbf{F}_{k}^{T})\cdot \mathbf{1}+\rho_2(\mathbf{w}^{k+1} - \mathbf{w}^{k}))\cdot \mathbf{z}\}
\end{align}

Similarly if we define $g(\mathbf{w},\mathbf{F}) = \mathbf{I}_{\mathcal{D}}(\mathbf{w},\mathbf{F})$ the optimality condition for the \emph{pair} of variables $(\mathbf{w},\mathbf{F})$, which form a $K\times (K+1)$ matrix is as follows.
% \begin{align} \label{optimalityCon21}
% 0 \in  %\mathcal{L}_{\rho_1,\rho_2}(\mathbf{z}^{k+1},\mathbf{w}^{k+1},\mathbf{F}^{k+1},\boldsymbol{\lambda}_{1}^{k},\boldsymbol{\lambda}_{2}^{k}) = 
% \partial g(\mathbf{w}^{k+1},\mathbf{F}^{k+1}) - \mathbf{1} \cdot \boldsymbol{\lambda}_{1}^{kT} - \boldsymbol{\lambda}_{2}^{k} + \rho_1(\mathbf{z}^{k+1} - \mathbf{F}^{T(k)} \cdot \mathbf{1} - \mathbf{p}_0) + \rho_2 (\mathbf{z}^{k+1} - \mathbf{w}^{k})
% \end{align}
\begin{align} \label{optimalityCon21}
0 \in \partial g(\mathbf{w}^{k+1},\mathbf{F}^{k+1}) - \mathbf{\Lambda}
\end{align}

where $\mathbf{\Lambda} = [\mathbf{1}\cdot \boldsymbol{\lambda}_1^{kT},\boldsymbol{\lambda}_2^{k}]$. If we carefully integrate this expression and use the multipliers' updates we get the following.

\begin{align} \label{wF_alsoMinimizes}
\mathbf{(w,F)}^{k+1} = \underset{\mathbf{[w,F]}}{\operatorname{argmin}}\{g(\mathbf{w,F}) -\mathbf{1}^{T} \cdot \mathbf{F}\cdot \boldsymbol{\lambda}_{1}^{k+1}-\mathbf{w}^{T} \cdot \boldsymbol{\lambda}_{2}^{k+1}\}
\end{align}

As $\mathbf{z}^{k+1}$ and $\mathbf{[w,F]}^{k+1}$ minimize the expressions in Eqs.(\ref{z_alsoMinimizes}) and (\ref{wF_alsoMinimizes}) they give a lower value for these expressions compared to $\mathbf{z}^{\ast}$ and $\mathbf{[w,F]}^{\ast}$ respectively, therefore we have the following two inequalities that upper-bound the differences of the v

\begin{align} \label{Ineq_f}
f(\mathbf{z}^{k+1}) - f(\mathbf{z}^{\ast}) \le 
\begingroup
\color{red}
\underbrace{\color{black}(\boldsymbol{\lambda}_{1}^{k+1}+\rho_1 \mathbf{1}^T \cdot (\mathbf{F}^{k+1} - \mathbf{F}^{k})}
\endgroup
 + \\ \nonumber
 \begingroup
\color{blue}
\underbrace{\color{black}\boldsymbol{\lambda}_{2}^{k+1} + \rho_2(\mathbf{w}^{k+1} - \mathbf{w}^{k})^{T})}
\endgroup
\cdot \begingroup
\color{green}
\underbrace{\color{black}(\mathbf{z}^{\ast} - \mathbf{z}^{k+1})}
\end{align}

\begin{align} \label{Ineq_g}
g(\mathbf{w,F}^{k+1}) - g(\mathbf{w,F}^{\ast}) \le
\begingroup
\color{red}
\underbrace{\color{black}\mathbf{1}^{T}\cdot(\mathbf{F}^{k+1} - \mathbf{F}^{\ast}) \cdot \boldsymbol{\lambda}_{1}^{k+1}}
\endgroup
+ \\ \nonumber 
\begingroup
\color{blue}
\underbrace{\color{black}(\mathbf{w}^{k+1} - \mathbf{w}^{\ast})^{T}\cdot \boldsymbol{\lambda}_{2}^{k+1}}
\endgroup 
\end{align}

Taking advantage of the following relations
\begin{itemize}
    \item $\mathbf{z}^{\ast} = \mathbf{1}^T \cdot \mathbf{F}^{\ast} + \mathbf{p}_0$
    \item $\mathbf{z}^{k+1} = \mathbf{r}_{1}^{k+1} +  \mathbf{F}^{(k+1)T} \cdot \mathbf{1} + \mathbf{p}_0$
\end{itemize}
The vector in green can be now rewritten as 
\begin{equation}
(\mathbf{z}^{\ast} - \mathbf{z}^{k+1}) = ( (\mathbf{F}^{\ast} - \mathbf{F}^{k+1})\cdot \mathbf{1} - \mathbf{r}_{1}^{k+1}).
\end{equation}

The above two inequalities will be eventually added, therefore we can group (add) the red terms of the two inequalities (along with the green term for the first one) and this expression will yield

\begin{equation} \label{expr-bef-adding1}
-\boldsymbol{\lambda}_{1}^{(k+1)T}\cdot
\mathbf{r}_{1}^{k+1} + \rho_1 \mathbf{1}^{T} \cdot (\mathbf{F}^{k+1} - \mathbf{F}^{k}) \cdot [- \mathbf{r}_{1}^{k+1} +  (\mathbf{F}^{\ast} - \mathbf{F}^{k+1})^{T}\cdot \mathbf{1}]
\end{equation}

Similarly to earlier, we have
\begin{itemize}
    \item $\mathbf{z}^{\ast} = \mathbf{w}^{\ast}$
    \item $\mathbf{z}^{k+1} = \mathbf{r}_{2}^{k+1} + \mathbf{w}^{k+1}$
\end{itemize}
The terms in blue will give us the following simplified expression
\begin{equation} \label{expr-bef-adding2}
-\boldsymbol{\lambda}_{2}^{(k+1)T}\cdot
\mathbf{r}_{2}^{k+1} + \rho_2 (\mathbf{w}^{k+1} - \mathbf{w}^{k})^{T} \cdot [- \mathbf{r}_{2}^{k+1} + (\mathbf{w}^{\ast} - \mathbf{w}^{k+1})]
\end{equation}

We have thus treated the RHSs of the Eqs.(\ref{Ineq_f},~\ref{Ineq_g}) which if we  add them we get the RHS of the second inequality of Lemma \ref{lemma:ineq}.
Finally, adding their LHSs will result to the scalar quantity $p^{k+1}-p^{\ast}$ which is the RHS of the aforementioned inequality. 

\myitem{Proof for inequality (\textit{a})}.
We multiply by two and add the two inequalities ($b,c$) to get the following one

\begin{align} \label{a3+a2}
    2(\boldsymbol{\lambda}_{1}^{k+1}-\boldsymbol{\lambda}_{1}^{\ast})^{T}\cdot \mathbf{r}_{1}^{k+1} + 2\rho_1 \mathbf{1}^T \cdot(\mathbf{F}^{k+1}- \mathbf{F}^{k})\cdot \mathbf{r}_{1}^{k+1}  \\ \nonumber -2\rho_1\mathbf{1}^{T} \cdot(\mathbf{F}^{k+1} -\mathbf{F}^{k}) \cdot(\mathbf{F}^{\ast} -\mathbf{F}^{k+1})^{T}\cdot \mathbf{1} \\ \nonumber
    + (\boldsymbol{\lambda}_{2}^{k+1}-\boldsymbol{\lambda}_{2}^{\ast})^{T}\cdot \mathbf{r}_{2}^{k+1} + \rho_2\cdot (\mathbf{w}^{k+1} - \mathbf{w}^{k})^{T}\cdot \mathbf{r}_{2}^{k+1}  \\ \nonumber - \rho_2 (\mathbf{w}^{k+1}- \mathbf{w}^{k})^{T}\cdot (\mathbf{w}^{\ast} - \mathbf{w}^{k+1}) \le 0
\end{align}

We first take a close look at the first two lines of Eq.(\ref{a3+a2}).
Substituting $\boldsymbol{\lambda}_1^{k+1} = \boldsymbol{\lambda}_1^{k}+\rho_1 \mathbf{r}_1^{k+1}$ and considering only the first term results to the following expression
\begin{equation} \label{multiplier1-and-res1}
2(\boldsymbol{\lambda}_1^{k}-\boldsymbol{\lambda}_1^{\ast})^{T}\cdot \mathbf{r}_1^{k+1} +\rho_1 ||\mathbf{r}_1^{k+1}||^2 + \rho_1 ||\mathbf{r}_1^{k+1}||^2
\end{equation}

We could further substitute $\mathbf{r}_1^{k+1}$ in the first two terms, keeping intact the last one.
\begin{equation} \label{r1:function}
\mathbf{r}_1^{k+1}=(1/\rho_1)(\boldsymbol{\lambda}_1^{k+1}- \boldsymbol{\lambda}_1^{k})
\end{equation}

We also use the fact that we can always write 
\begin{equation} \label{eq:dimotiko}
\boldsymbol{\lambda}_1^{k+1}-\boldsymbol{\lambda}_1^{k} = (\boldsymbol{\lambda}_1^{k+1}-\boldsymbol{\lambda}_1^{\ast}) - (\boldsymbol{\lambda}_1^{k}-\boldsymbol{\lambda}_1^{\ast})
\end{equation}

Combining Eqs.(\ref{r1:function},~\ref{eq:dimotiko}) and plugging them in Eq.(\ref{multiplier1-and-res1}) will give us
\begin{equation} \label{multipliers1:big-ineq}
(1/\rho_1)(||\boldsymbol{\lambda}_1^{k+1}-\boldsymbol{\lambda}_1^{\ast}||^2-||\boldsymbol{\lambda}_1^{k}-\boldsymbol{\lambda}_1^{\ast}||^2)+\rho_1||\mathbf{r}_1^{k+1}||^2
\end{equation}

To treat the remaining terms of the first two lines of \ref{a3+a2}, we do the following substitution
\begin{equation}
\mathbf{F}^{k+1}-\mathbf{F}^{\ast}= (\mathbf{F}^{k+1}-\mathbf{F}^{k}) - (\mathbf{F}^{k}-\mathbf{F}^{\ast})
\end{equation}

If we also open the multiplicative brackets, we get
\begin{align}\label{eq:unimpo}
\begingroup
\color{green}
\underbrace{\color{black}\rho_1||\mathbf{r}_1^{k+1}||^2 + 2\rho_1 \mathbf{1}^T\cdot(\mathbf{F}^{k+1}-\mathbf{F}^{k})\cdot \mathbf{r}_{1}^{k+1}}
\endgroup + \\ \nonumber  
\begingroup
\color{red}
\underbrace{\color{black}2\rho_1(\mathbf{1}^T\cdot(\mathbf{F}^{k+1}-\mathbf{F}^{k})(\mathbf{F}^{k+1}-\mathbf{F}^{k})^{T} \cdot \mathbf{1}}
\endgroup
  \\ \nonumber 
- 2 \rho_1 \mathbf{1}^T \cdot(\mathbf{F}^{k+1}-\mathbf{F}^{k})\cdot
\begingroup
\color{red}
\underbrace{\color{black}(\mathbf{F}^{k}-\mathbf{F}^{\ast})^{T}}
\endgroup
\cdot \mathbf{1}
\end{align}

The red expression in the middle line of Eq.(\ref{eq:unimpo}) above can be rewritten as 
\begin{equation} \label{dotProduct2norm}
2\rho_1||\mathbf{1}^{T}\cdot(\mathbf{F}^{k+1}-\mathbf{F}^{k})||^2    
\end{equation}

The expression in (\ref{dotProduct2norm}) comes handy, as it allows us complete the square identity with the green underlined expression.
\begin{align}
\rho_1||\mathbf{r}_1^{k+1} + \mathbf{1}^{T} \cdot  (\mathbf{F}^{k+1}-\mathbf{F}^{k})||^2 + & \rho_1|| \mathbf{1}^{T} \cdot  (\mathbf{F}^{k+1}-\mathbf{F}^{k})||^2 - \\ \nonumber
 2\rho_1 \mathbf{1}^{T} \cdot  (\mathbf{F}^{k+1}-\mathbf{F}^{k})\cdot (\mathbf{F}^{k}-\mathbf{F}^{\ast})^{T}\cdot \mathbf{1}
\end{align}

We do one last substitution in the last two terms of the above expression of the form
\begin{equation}
\mathbf{F}^{k+1}-\mathbf{F}^{k}= (\mathbf{F}^{k+1}-\mathbf{F}^{\ast}) - (\mathbf{F}^{k}-\mathbf{F}^{\ast})
\end{equation}

This will finally give us 
\begin{align} \label{F:big-ineq}
&\rho_1||\mathbf{r}_1^{k+1} + \mathbf{1}^{T} \cdot  (\mathbf{F}^{k+1}-\mathbf{F}^{k})||^2 + 
\rho_1(||\mathbf{1}^{T} \cdot  (\mathbf{F}^{k}-\mathbf{F}^{\ast})||^2 - \\ \nonumber
&||\mathbf{1}^{T} \cdot  (\mathbf{F}^{k+1}-\mathbf{F}^{k})||^2)
\end{align}

Following the exact same reasoning we did for the first two lines of Eq.(\ref{a3+a2}), we do the same for the two last lines. This suggests the term corresponding to them multipliers of the third line (\ref{a3+a2}) will be written as

\begin{equation} \label{multipliers2:big-ineq}
(1/\rho_2)(||\boldsymbol{\lambda}_2^{k+1}-\boldsymbol{\lambda}_2^{\ast}||^2-||\boldsymbol{\lambda}_2^{k}-\boldsymbol{\lambda}_2^{\ast}||^2)+\rho_2||\mathbf{r}_2^{k+1}||^2
\end{equation}

While the remaining terms of the last two lines of Eq.(\ref{a3+a2}) can be similarly written as
\begin{align} \label{w:big-ineq}
\rho_2||\mathbf{r}_2^{k+1} +  (\mathbf{w}^{k+1}-\mathbf{w}^{k})||^2 +
\rho_2(|| (\mathbf{w}^{k}-\mathbf{w}^{\ast})||^2 - 
 ||(\mathbf{w}^{k+1}-\mathbf{w}^{k})||^2)
\end{align}
% \begin{equation}
% V_k^{1} = \frac{1}{\rho_1} ||\boldsymbol{\lambda}_{1}^{k} - \boldsymbol{\lambda}_{1}^{\ast} ||^2 + \rho_1 ||\mathbf{1}^T \cdot (\mathbf{F}^{k+1} -\mathbf{F}^{k} )||^2 \end{equation}
% \begin{equation}
% V_k^{2} = \frac{1}{\rho_2} ||\boldsymbol{\lambda}_{2}^{k} - \boldsymbol{\lambda}_{2}^{\ast} ||^2 + \rho_2 ||\mathbf{z}^{\prime(k+1)} -\mathbf{z}^{\prime(k) }||^2.
% \end{equation}

Observing the definition of the Lyapunov function $V_k$, and using our main Eq.(\ref{a3+a2}) along with the use of expressions (\ref{multipliers1:big-ineq},\ref{F:big-ineq}) and (\ref{multipliers2:big-ineq},\ref{w:big-ineq}) we have
\begin{align} \label{w:big-ineq}
V_k - V_{k+1} \ge \rho_1||\mathbf{r}_1^{k+1} +  \mathbf{1}\cdot(\mathbf{F}^{k+1}-\mathbf{F}^{k})||^2 + \\ \nonumber
\rho_2(||\mathbf{r}_2^{k+1} +  (\mathbf{w}^{k+1}-\mathbf{w}^{k})||^2)
\end{align}

To prove Eq.(\textit{a}) from Lemma~\ref{lemma:ineq}, it is enough to show that the two middle terms of the expanded squared norms are positive. Namely that

\begin{equation} \label{target:ineq}
-2\rho_1 \mathbf{r}_1^T \cdot (\mathbf{F}^{k+1}-\mathbf{F}^{k})^{T}\cdot \mathbf{1} -2 \rho_2 \mathbf{r}_2^T \cdot (\mathbf{w}^{k+1} - \mathbf{w}^{k})\ge 0
\end{equation}

We remind that $(\mathbf{w}^{k+1},\mathbf{F}^{k+1})$ and $(\mathbf{w}^{k},\mathbf{F}^{k})$ minimize the respective expressions
\begin{equation}
g(\mathbf{w,F}) -\mathbf{1}^{T} \cdot \mathbf{F}\cdot \boldsymbol{\lambda}_{1}^{k+1}-\mathbf{w}^{T} \cdot \boldsymbol{\lambda}_{2}^{k+1}
\end{equation}
\begin{equation}
g(\mathbf{w,F}) -\mathbf{1}^{T} \cdot \mathbf{F}\cdot \boldsymbol{\lambda}_{1}^{k}-\mathbf{w}^{T} \cdot \boldsymbol{\lambda}_{2}^{k}
\end{equation}

This allows us to write the following two inequalities.
\begin{align} \label{ineq:reminder1}
&g(\mathbf{w}^{k+1},\mathbf{F}^{k+1}) - \mathbf{1}^{T}\cdot\mathbf{F}^{k+1}\cdot\boldsymbol{\lambda}_1^{k+1} - \mathbf{w}^{T(k+1)}\cdot\boldsymbol{\lambda}_2^{k+1} \le \\ \nonumber
&g(\mathbf{w}^{k},\mathbf{F}^{k}) - \mathbf{1}^{T}\cdot\mathbf{F}^{k}\cdot\boldsymbol{\lambda}_1^{k+1} - \mathbf{w}^{T(k)}\cdot\boldsymbol{\lambda}_2^{k+1}
\end{align}

\begin{align} \label{ineq:reminder2}
&g(\mathbf{w}^{k},\mathbf{F}^{k}) - \mathbf{1}^{T}\cdot\mathbf{F}^{k}\cdot\boldsymbol{\lambda}_1^{k} - \mathbf{w}^{T(k)}\cdot\boldsymbol{\lambda}_2^{k} \le \\ \nonumber
&g(\mathbf{w}^{k},\mathbf{F}^{k}) - \mathbf{1}^{T}\cdot\mathbf{F}^{k}\cdot\boldsymbol{\lambda}_1^{k+1} - \mathbf{w}^{T(k)}\cdot\boldsymbol{\lambda}_2^{k+1}
\end{align}

Adding the Eqs.(\ref{ineq:reminder1},\ref{ineq:reminder2}), results the following single inequality
\begin{align} \label{final:ineq}
\mathbf{1}^T \cdot (\mathbf{F}^{k+1}-\mathbf{F}^{k+1})\cdot (\boldsymbol{\lambda}_1^{k+1} - \boldsymbol{\lambda}_1^{k}) + \\ \nonumber (\mathbf{w}^{k+1}-\mathbf{w}^{k})^{T}\cdot (\boldsymbol{\lambda}_2^{k+1}-\boldsymbol{\lambda}_2^{k}) \ge 0
\end{align}

For both differences of multipliers we substitute $\rho_i \mathbf{r}_i^{k+1} = \boldsymbol{\lambda}_i^{k+1}-\boldsymbol{\lambda}_i^{k}$

Plugging the last substitution to Eq.(\ref{final:ineq}), we see that in order for Eq.(\ref{target:ineq}) to hold is to require $\rho_1,\rho_2 \ge 0$.
